# Supplementary material for: Memory Is All You Need: Testing How Model Memory Affects LLM Performance in Annotation Tasks
Source: arXiv:2503.04874 source file (2025-03-06)
Supplement: Supplementary file 1 [file appendix.pdf]

## Appendix for: “Memory Is All You Need”


**A Reward and Punishment Prompts** **2**

**B The Costs, Limits and Time of Running LLMs** **3**

**C Few-shot Learning vs. No-Restart and Reinforcement** **5**

## Appendix A: Reward and Punishment Prompts

In the main manuscript we describe memory reinforcement, a prompting approach where the model is shown a text to classify, and then the researcher informs the model whether it was correct or not, sending a punishment or reward message. After the model provides a correct response to the classification task, it would see the following reward message:

> Congratulations, your classification was correct! Remember this for future classifications.

After the model provides an incorrect response to the classification task, it would see the following reward message:

> Unfortunately, your classification was incorrect. It should be: [expected label]. Try again to classify it, and remember to update your knowledge for future classifications.

## Appendix B: The Costs, Limits and Time of Running LLMs

In our tests, we find that Llama 3.1 tends to run faster than GPT-4o and rarely yields an API error. It is also cheaper when deployed through a web server like `deepinfra.com`.[1] Llama 3.1 is free when deployed locally, yet the hardware required to do so makes it an unrealistic option for many researchers. As Table B1 shows, the most expensive technique is *memory reinforcement*, as the number of input tokens increases with every run at a higher rate than with *memory prompting* (both OpenAI and DeepInfra charge by the input and output token). The differences in cost between Llama 3.1 and GPT-4o are stark. For example, with the 600 observations from the incivility dataset, running memory reinforcement would cost $12.63 with GPT-4o and $2.67 with Llama 3.1. Similarly, to run the same dataset with the same technique would take GPT-4o around 31 minutes, while it only takes Llama around 7 minutes. In both cases, however, the time to label the data is considerably lower than what it would take a human coder. Overall, considering costs, time, and performance, Llama seems to be the best option. However, testing the performance of both models with both memory approaches when using them in applied research should be within reach for many researchers.

As for rate limitations, Llama 3.1 has none while GPT-4o varies according to usage tiers – usage based on the amount of money spent on the platform. At Tier 1 ($5 paid), 500 calls per minute and 30,000 tokens per minute; at Tier 2 ($50 paid), 5,000 calls per minute and 450,000

| Model | Prompting Strategy | Case | Avg. Time (minutes) | Cost USD$ (per run) |
|---|---|---|---|---|
| GPT-4o | Zero-Shot No-Memory | Incivility | 6.15 | $0.10 |
| GPT-4o | Few-Shot No-Memory (CoT) | Incivility | 5.85 | $1.01 |
| GPT-4o | Memory Prompting | Incivility | 14.87 | $14.52 |
| GPT-4o | Memory Reinforcement | Incivility | 30.53 | $12.63 |
| Llama 3.1-70b | Zero-Shot No-Memory | Incivility | 2.2 | <$0.01 |
| Llama 3.1-70b | Few-Shot No-Memory (CoT) | Incivility | 2.42 | <$0.01 |
| Llama 3.1-70b | Memory Prompting | Incivility | 5.58 | $0.45 |
| Llama 3.1-70b | Memory Reinforcement | Incivility | 6.86 | $2.67 |
| GPT-4o | Zero-Shot No-Memory | Nostalgia | 5.326 | $0.11 |
| GPT-4o | Few-Shot No-Memory (CoT) | Nostalgia | 6.72 | $1.09 |
| GPT-4o | Memory Prompting | Nostalgia | 12.12 | $15.87 |
| GPT-4o | Memory Reinforcement | Nostalgia | 29.13 | $13.8 |
| Llama 3.1-70b | Zero-Shot No-Memory | Nostalgia | 4.48 | <$0.01 |
| Llama 3.1-70b | Few-Shot No-Memory (CoT) | Nostalgia | 5.03 | <$0.01 |
| Llama 3.1-70b | Memory Prompting | Nostalgia | 5.92 | $0.49 |
| Llama 3.1-70b | Memory Reinforcement | Nostalgia | 7.98 | $2.89 |

**Table B1:** Cost and time for each run, per model and dataset.

[1] This is the service we used to run our Llama models. The model is free but the server charges by the token at very low rates, as Table B1 shows. Researchers can use Llama locally for free or through a service such as this one.

tokens per minute; at Tier 3 ($100 paid), 5,000 calls per minute and 800,000 tokens per minute. When running *memory reinforcement*, we used ∼90M input tokens 7.921 output tokens over 10 runs and 310 minutes. We found that the rate limitations from OpenAI did not affect our pipeline after Tier 3. However, these limits may affect researchers who spend smaller amounts on the platform, especially with tasks that require sending long texts or conversation histories to the API.

## Appendix C: Few-shot Learning vs. No-Restart and Reinforcement

This appendix further compares few-shot learning CoT with memory prompting and memory reinforcement. First, we add the few-shot CoT prompt to both the original prompts for memory prompting and memory reinforcement. We do this to rule out that few-shot could further improve model performance. The most relevant result in Table C1, using the incivility dataset, is that including a few-shot prompt does not improve on the main results from the memory prompting and memory reinforcement approaches in Tables 2 and 3. In the case of Llama 3.1, memory reinforcement with zero-shot remains the clear best performer (see Table 2b in the main article).

**(a)** GPT-4o

| | Few-shot Memory Prompting | | | | Few-shot Memory Reinforcement | | | |
|---|---|---|---|---|---|---|---|---|
| | Prec. | Rec. | $F1$ | $SD_{F1}$ | Prec. | Rec. | $F1$ | $SD_{F1}$ |
| Civil | 0.886 | 0.775 | 0.827 | 0.008 | 0.911 | 0.724 | 0.807 | 0.009 |
| Uncivil | 0.800 | 0.900 | 0.847 | 0.005 | 0.771 | 0.929 | 0.843 | 0.003 |
| Overall | 0.843 | 0.837 | 0.837 | 0.006 | 0.841 | 0.826 | 0.825 | 0.006 |

**(b)** LLaMA 3.1

| | Few-shot Memory Prompting | | | | Few-shot Memory Reinforcement | | | |
|---|---|---|---|---|---|---|---|---|
| | Prec. | Rec. | $F1$ | $SD_{F1}$ | Prec. | Rec. | $F1$ | $SD_{F1}$ |
| Civil | 0.873 | 0.733 | 0.796 | 0.010 | 0.915 | 0.731 | 0.813 | 0.010 |
| Uncivil | 0.770 | 0.893 | 0.827 | 0.006 | 0.776 | 0.932 | 0.847 | 0.005 |
| Overall | 0.821 | 0.813 | 0.811 | 0.007 | 0.846 | 0.832 | 0.830 | 0.007 |

**Table C1:** Few-shot learning incivility results for the three different interaction approaches, by LLM.

Second, we also tested a variant of our reinforcement approach stripped of the reinforcement step, which would make the test equivalent to a few-shot learning approach with 120 examples. The results, as expected, are significantly worse than the original memory reinforcement approach, as few-shot learning is known to decrease performance with larger numbers of examples (**?**). Average performance losses range between 20 and 40 percent when compared to memory reinforcement, depending on model and dataset. This result also strengthens the value of the reinforcement step, as it does not appear to induce any of the issues related to adding too many examples to a few-shot prompt.
